# Supplementary material for: Secure Optimization Through Opaque Observations
Source: arXiv:2101.06039 source file (2021-01-15)
Supplement: Supplementary file 1 [file appendix.tex]

\section{Outline/TODO list.}

Proposition de plan
1) Intro
2) Related work
3) motivating example
4) Definition et background
4.1 - Mini IR + definition basique -- trace, event, tranformation correct
4.2 -- DEfinition des effets voulus -- preservation prop observable + preservation use de calcul
5) Mecanisme de préservation
5.1 -- Element basique : opaque, observe, ...
5.2 -- Macro les utilitisant pour préserver ce qu'on veut
et on explique avec les mains ou les piedds que ca fait ce qu'on veut
6) Implementation dans LLVM
IR + back-end avec optimisation 
7) Experimentations

TODO: model atomic and/or join using existing relations, but how? Herding Cats does not seem to help much on atomic read-modify-write (RMW) operations.

Probably deprecated note: I agree to eliminate the dd relation in favor of an intra-instruction causality order iico among finer grain events, if this happens to be easier to manage (see Herding Cats for example).

TODO: add implementation of MiniIR into LLVM (using opaque or tokenize, and optional side-effects) and discuss informally its correctness w.r.t. OF Preservation.

\section{SSA Syntax}

Note 1: if conditionals, while loops and atomic expressions break the linear CFG of LLVM IR, introducing a limited form of structure with nested regions. Conditionals and loops are provided for
simplification purposes, but (we believe) this does not hide any significant difficulty with extending our approach to general control flow. Atomic regions (or join operations) are an essential feature and
may be implemented in a linear CFG like LLVM IR by means of intrinsics and/or inline assembly (with a dedicated translation table to be provided).

(CG) Agree, we can abstract away control flow and reason on valid IR traces, because for now we do not propose anything related to control flow, for the proofs we just need to reason about instructions
sequences (atomic or not) with incoming values for which we do not see the reaching definitions. Of course at C level we will have to introduce C-syntax sequence points and what they imply for the partial
schedule of the users annotations and (non-uniques) variables definitions if needed

(AC) agreed.

Note 2: There are no program points in the partial observation trace. C labels may be used to derive abstract values (tokens, locations in Christophe's words) or alternatively, (file, line) pairs just like
dwarf debug info would do.

(CG) Not sure to understand if you mean label == location. It is not. For me a "location" is an abstract identifier for representing a (name, value) pair. In my examples I added C labels just for the
examples as a shortcut for saying at C level: "the name X at this source file/line", The abstract location being the value : ("the name x at this source file/line", value of x). I admit that location is
not a good name, but it is not an address, it is a unique identity for the (name,value) pair at this program point. If the user do not care about le source file/line (for instance because there is no
ambiguity on what is the original name "x", The pair can be ("x", value of x). It is not the case in general.

(AC) agreed and fixed.

Note 3: banning the "location" terminology of the CC paper, in favor of the less ambiguous "address".

TODO Note: consider adding a no-preservation-guarantee annotate(var, "...") and instruction annotation string. It is meant to be present in the partial observation trace if it got preserved down to the
binary, but with no guarantee.

\section{Axiomatic relations}
Let us define an abstract axiomatic semantics of our Mini IR. It is abstract in the sense that it refers to the semantics of explicit observations only. Note that these axiomatic relations hold on
instructions, not on uses or definitions.
\begin{itemize}
  \item Def-Use relation:
  \begin{align*}
    \mathit{DI} \xrightarrow{du} \mathit{UI} \mid \mathit{DI} & \text{ instruction defining a value } v,\\
                                                  \mathit{UI} & \text{ instruction using } v
  \end{align*}
  \item Def-Def relation:
  \begin{align*}
    \mathit{DI} \xrightarrow{dd} \mathit{DI'} \mid \mathit{DI} & \text{ instruction defining a value } v,\\
                                                   \mathit{DI'} & \text{ instruction using } v \text{ to define a new value } v'
  \end{align*}
(SV) This second one seems redundant to me. What's crucial here to ensure the happens before relation between di' and di is the fact that di' uses v, so basically this falls into the def-use relation doesn't it?

(AC) I should have added a comment... this rule is very misleading indeed, and due to the fact all relations hold on instructions rather than individual uses and defs. I wanted to capture the fact that the
definition in the LHS of an instruction happens after the uses in the RHS of this instruction! This is what this rule cumbersomely achieves, if I am not mistaken.

(AG) I don't understand this rule: unless anti-causal IR is in use (which I have never seen in practice), one can not define a value without using the values needed to define it (there is a dataflow
dependency here).  I guess what you want to express is the "happens-before" relation between 2 instructions without the usual dependency (i.e. register, memory or side-effect) already well managed by
compilers.

(CG) I guess that once you've introduced what is an SSA-instruction and said that an instruction reads variables values and constant values on the RHS, then computes some functions of these values, and then store the results in some variables in the LHS, it is sufficient.

(AC) this is what it says, talking about instructions only (i.e., not talking about uses and defs, but I agree it is confusing).

(CG) If we use some of the terminology used in Batty et al. (Mathematizing C++ Concurrency) the def-use relation if also called the "read-from (rf)" (i.e. there is noredefinition of v in-between) relation between the instructions

(AC) it is related, but rf is for memory and and comes later in the list, memory models don't care much about def-use (only control dependences for Power/ARM), the distinction is important.

(CG) The RHS is evaluated before the stores in LHS, is that RHS reads are "sequenced-before" LHS writes (like the sequence point in C at '=') and each RHS is data-dependent of all LHS, but in their cases, as
the reasoning is on operations that write/read mem, (and hence does not both read and write registers).

(AC) sb would also make sense here, I agree. Maybe better than dd. I'll think about it.

(CG) Thus back to your SSA-instructions, just define that it reads from all RHS before it writes to all LHS, i.e. reads happen-before writes, each RHS var is data-dependent of all LHS vars. In the MinIR (the
minir.org work with Julien Leguen), I implemented each instruction as a parallel assignment to some operands or memory slice of some expression trees over operands and memory slice values, hence all reads
happen-before all writes and each write data-depends on some reads (or all by defaut if the semantic is unknown).

(AC) Thanks for reminding me of MinIR I knew the name sounded familiar when Son/Karine/Arnaud mentionned we should have one but did not resurface your work with Julien (and Fabrice ?) until now! We shouild
cite it in MLIR's next paper (nothing moved since the arXiv paper in February...)
  \item Hide-Value relation: TODO add a weaker pre-eval relation and syntax (more abstract than opaque), with a compilation rule lowering pre-eval to opaque in compilers where hiding through an opaque value is the natural
  way to enforce pre-evaluation.
  \begin{align*}
    \mathit{DI} \xrightarrow{hv} \mathit{UI} \mid \mathit{DI} & \text{ instruction defining a value } v,\\
                                                  \mathit{UI} & \text{ instruction involving } v \text{ through an opaque use of } v
  \end{align*}
(CG) for the pre-evaluation case, note that this is too strong, but we can prove that opaque implies pre-eval, we should probably try to define pre-eval 
  \item Read-From relation: (RAW?) TODO explain the reaching definition meaning of rf w.r.t. raw and double-check this is the classical usage in memory models

(CG) Batty defines it from the sequence points (that we can assume resolved) and the fact that there is no redef of the variable in between (happens-before-hidden)

(AC) Thanks. This is the standard "last write" or "value-based dependence" or "array dataflow" or "instancewise reaching definition" definition then (different loop nest/array terminologies for the same thing, a mess...).

(CG) Also  I guess that read-from is interesting and may also apply to registers in our case. This is realy what enforces data-dependency (implying happens-before in the trace) between your operations (see
above). Indeed, in my intrincics (which are at an higher abstraction level), I do not distinguish memory or register objects, hence for me there is a read-from dependency in both cases.

(AC) We need to distinguish it from the du relation, but I agree rf implies the presence of a du from the instruction that defines the value stored in memory to its use in the rf relation. This is important for the fine-tuning of the hb relation.
  \begin{align*}
    \mathit{SI} \xrightarrow{rf} \mathit{LI} \mid \mathit{SI} & \text{ instruction storing to } \mathit{addr},\\
                                                  \mathit{LI} & \text{ instruction loading from } \mathit{addr}
  \end{align*}
  \item WAW relation
  \item WAR relation
  \item Observe-From relation:
  \begin{align*}
    \mathit{SI} \HBOF \mathit{OI} \mid \mathit{SI} & \text{ instruction storing to } \mathit{addr},\\
                                                  \mathit{OI} & \text{ instruction observing } \mathit{addr}
  \end{align*}
(CG) at this level, I guess that the observe must be indeed a specific operator, which implies a read-from relationship with some previous instruction through it's RHS operands. We need, I think introduce
the observe-from relationship (and its transitive closure) which is for the "monitor", no problem if for the program (or monitor) there is also a read-from. Indeed. In my primitives proposal, actually, there
is a read-from relationship from the location id, and actually the expose operation is an observe-from the parameters of the expose (the name.value pair). Hence I have a read-from some arbitrary id at the
property observation point, while the monitor will observe-from the exposed pair (earlier in the trace) for each variable. Hence at the observation point, we have a closure of read-from and observe-from
which makes and observe-from* and the monitor can evaluate the expression. 

TBC. Certainly missing some. See herding cats paper for examples and inspiration, and check Christophe's use cases.
\end{itemize}

\subsection{Compiler enforcement of observation axioms}
Compiler passes may or may not enforce relations among instructions, among variables and memory locations. Their soundness is defined w.r.t. to a happens-before relation hb that may depend on the compiler pass.

Some passes assume opaque data flow and side-effects:

    hb = du, dd, hi, rf, waw, war, of

    Basic block or global scheduling (without common subexpression elimination).

    TODO: list more passes.

Some passes analyze concrete expressions and their equivalence or possible simplifications:

    hb = hi, rf, waw, war, of

    E.g., GVN/CSE/PRE of pure expressions, expression folding, strength reduction, loop unrolling (update and simplification of IVs).

    TODO: list more passes and be more specific about what alternate/weaker relations may hold instead of du and dd, introducing these if necessary.

Some passes relax memory ordering leveraging analyses of side-effects:

    hb = du, dd, hi, of

    E.g., memtoreg, CSE of loads and stores, polly.

    TODO: list more passes and be more specific about the relaxation, possibly introducing more relations such as memory dependences.

Some passes relax memory ordering and also analyze concrete expressions:

    hb = hi, of

    E.g., vectorization and polly with support for reductions.

TBC. Probably missing relations necessary to prove the preservation of observational semantics in more advanced transformations such as those reasoning on concrete values (GVN/CSE/PRE of pure expressions,
expression folding) or those reasoning on precise side-effect information (CSE of loads and stores, polly). If such relations are missing, they are also likely to limit our ability to prove that
observe/opaque/atomic preserve anything.

(SV) IIUC, the goal here is to list every (or at least as many as we can) existing compiler transformation and try to prove that it respects the hb relation of hi and of? Does it mean we lose generality
here, since we have to do this transformation by transformation? I certainly am missing something here...

(AC) This is absolutely correct. We do not lose generality in defining the hb relation itself, but we do lose generality in proposing multiple variants of hb, more or less constraining in terms of optimizing
power of the authorized transformations.

(AG) I think this is missing the point here (or I am completely lost): the goal is to rely on existing relations already well managed by the compiler (so we don't have to mofify passes): how does 'of' differs
from 'rf' (apart that 'rf' may have no use... and needs either to be side-effecting, or return a value that can be used and needs to be hooked somewhere else, refer to last call discussions). To be clear en
comforting: I like those 2 sections. But I think they should be re-organized. On one hand, there are the standard axioms (terminal axioms ?) that every compiler will fulfill. Then we have our 2 axioms (of
and hi). As 'of' and 'hi' can be implemented in terms of terminal axioms, any standard compiler will respect the axioms. No need to modify the compiler or the passes to teach them about the new axioms. QED.

(AC) I agree with Arnaud's point. We need to distinguish two levels: proving properties/correctness of transformations w.r.t. the axiomatic relations, separately from defining correct/conservative implementations of the code-fragments/builtins implementing those relations (observe, opaque, atomic/join).

\subsection{Examples of primitives}
A misnomer as these primitives are actually implemented using the syntax above. We strive to reduce unnecessary atomicity and opacity thereby relaxing constraints on the valid program transformations.

Note 1: program transformations may be required on top of these primitives to enforce functional properties as defined in Vu et al. CC 2020.

Note 2: instead of relying on specific program transformations, one may complement these primitives with appropriate coding rules associated with every functional property, as proposed by Christophe.

\begin{itemize}
  \item Join: returning the first value (note, it used to be a dummy value but this variant is more powerful and cheaper)
  \begin{lstlisting}
macro join(v1, ..., vk) {
  u1, ..., uk = atomic {  ; alternatively, this single region catching 
                          ; all variables may be decomposed into a log-tree 
                          ; of pairwise atomic regions 
                          ; (not sure if this has any practical benefits)
    yield(v1, ..., vk)
  }
  return(u1)
}
  \end{lstlisting}

  \item Side-effecting join
  \begin{lstlisting}
macro side_effecting_join(v1, ..., vk, abstract_addr) {
  u1, ..., uk = atomic read(abstract_addr) write(abstract_addr) { 
     ; alternatively, this single region catching 
     ; all variables may be decomposed into a log-tree 
     ; of pairwise atomic regions 
     ; (not sure if this has any practical benefits)
    mem[abstract_addr] <- dummy_value 
     ;  Do we really need this ? 
     ; The use of a dummy_value looks bad. 
     ; Agreed, an opaque store would be better. 
     ; Thinking about it but the instruction cannot simply be removed.
    observe(abstract_addr)

    yield(v1, ..., vk)
  }
  return(u1)
}
  \end{lstlisting}

  \item Barrier: renaming all variables. TODO(albert) revisit the Dekker or Peterson mutex algorithms with phi nodes to simulate atomic with plain SSA, this would be a major discovery (i.e., no inline asm or
  intrinsic or any out-of-dataflow world all-powerful god needed), I mentioned this months ago as a joke but it may actually be possible. Dekker is more likely to work because it does not involve concurrent
  write, while Peterson does.
  \begin{lstlisting}
macro barrier(v1, ..., vk) {
  u1, ..., uk = atomic {  ; alternatively, this single region catching 
                          ; all variables may be decomposed into a log-tree 
                          ; of pairwise atomic regions 
                          ; (not sure if this has any practical benefits)
    yield(v1, ..., vk)
  }
  return(u1, ..., uk)
}
  \end{lstlisting}

  \item Side-effecting barrier
  \begin{lstlisting}
macro side_effecting_barrier(v1, ..., vk, abstract_addr) {
    u1, ..., uk = atomic readwrite(abstract_addr) {
    mem[abstract_addr] <- dummy_value
    observe(abstract_addr)

    yield(v1, ..., vk)
  }

  return(u1, ..., uk)
}
  \end{lstlisting}

  \item CC's observation: Side-effecting observation and renaming, no join point, broken down into individual atomic regions corresponding to Son's observation intrinsic
  \begin{lstlisting}
macro observation_point_CC(v1, ..., vk) {
  w1 = opaque(v1)
  ...
  wk = opaque(vk)

  u1 = atomic readwrite(common_abstract_addr_to_all_observation_points) {
    observe(w1)
    mem[common_abstract_addr_to_all_observation_points] <- dummy_value
    observe(common_abstract_addr_to_all_observation_points)
    yield(w1)  ; opaque value
  }
  ...
  uk = atomic readwrite(common_abstract_addr_to_all_observation_points) {
    observe(wk)
    mem[common_abstract_addr_to_all_observation_points] <- dummy_value
    observe(common_abstract_addr_to_all_observation_points)
    yield(wk)
  }

  return(u1, ..., uk)
}
  \end{lstlisting}

  \item CC's observation: Side-effecting observation and renaming, no join point, broken down into individual atomic regions corresponding to Son's observation intrinsic
  \begin{lstlisting}
macro observation_point_CC(v1, ..., vk) {
  w1 = opaque(v1)
  ...
  wk = opaque(vk)

  u1 = atomic readwrite(common_abstract_addr_to_all_observation_points) {
    observe(w1)
    mem[common_abstract_addr_to_all_observation_points] <- dummy_value
    observe(common_abstract_addr_to_all_observation_points)
    yield(w1)  ; opaque value
  }
  ...
  uk = atomic readwrite(common_abstract_addr_to_all_observation_points) {
    observe(wk)
    mem[common_abstract_addr_to_all_observation_points] <- dummy_value
    observe(common_abstract_addr_to_all_observation_points)
    yield(wk)
  }

  return(u1, ..., uk)
}
  \end{lstlisting}

  \item Exposition:
  \begin{lstlisting}
macro expose_val(v) {
  u = opaque<unit>(v)  ; u is of type 'unit', opaque to 
                       ; CSE, PRE, GVN, constant propagation, folding, etc., 
                       ; and not involving any storage requirements at 
                       ; and after regalloc.
  return(u)
}
  \end{lstlisting}

  \item Exposition map: Rename to unit type then join atomically over multiple variables, forcing uses of the renamed variables to occur after all observations
  \begin{lstlisting}
macro expose_map(v1, ..., vk) {
  u1 = expose_val(v1)
  ...
  uk = expose_val(vk)
  w = join(u1, ..., uk)

  return(w)
}
  \end{lstlisting}

  \item Exposition prop: Observe and rename over all variables of a property, then evaluate it, observe and rename its result
  \begin{lstlisting}
macro expose_prop('prop(`v1, ..., `vk)') {
  p = eval 'prop(`v1, ..., `vk)'  ; quasi-quotation syntax for the evaluation of functional properties

  return(p)
}
  \end{lstlisting}

The implementations below rely on atomic. I'm now increasingly tempted to redefine them in terms of join instead. Moving everything to join-based implementations, which would be faithful to both approaches of Son (unary/elementary primitivies) and Christophe (relax constraints as much as possible for best performance). More likely we should have both join-based and atomic-based implementations and discuss/compare them in the paper and experiments.

  \item Observe: Observe and rename atomically, forcing uses of the renamed variable to occur after the observation
  \begin{lstlisting}
macro observe_val(v) {
  u = atomic {
    observe(v)
    yield(v)
  }
  return(u)
}
  \end{lstlisting}

  \item Observe map: Observe and rename atomically per variable, then joining atomically over multiple variables, forcing uses of the renamed variables to occur after all observations => how to formally
  express the fact that subsequent uses of v1, ..., vk now use w1, ... wk
  \begin{lstlisting}
macro observe_map(v1, ..., vk) {
  u1 = atomic {
    observe(v1)
    yield(v1)
  }
  ...
  uk = atomic {
    observe(vk)
    yield(vk)
  }

  w1, ..., wk = barrier(u1, ..., uk)

  return(w1, ..., wk)
}
  \end{lstlisting}

  \item Observe prop: Observe and rename over all variables of a property, then evaluate it, observe and rename its result
  \begin{lstlisting}
macro observe_prop('prop(`v1, ..., `vk)) {
  u1 = atomic {
    observe(v1)
    yield(v1)
  }
  ...
  uk = atomic {
    observe(vk)
    yield(vk)
  }

  p = eval 'prop(`u1, ..., `uk)'  ; quasi-quotation syntax for the evaluation of functional properties
  observe(p)

  return(p)
}
  \end{lstlisting}

  \item Another observe...: Observe and rename over all variables of a property, then evaluate it, observe and rename its result, ordered through a side-effect
  \begin{lstlisting}
macro observe_prop_state('prop(`v1, ..., `vk)') {
  u1 = atomic {
    observe(v1)
    yield(v1)
  }
  ...
  uk = atomic {
    observe(vk)
    yield(vk)
  }

  w1, ..., wk = side_effecting_barrier(u1, ..., uk)

  p = eval 'prop(`w1, ..., `wk)'  ; quasi-quotation syntax for the evaluation of functional properties
  observe(p)

  return(p)
}
  \end{lstlisting}

  \item Rename and hide
  \begin{lstlisting}
macro enforce_val(v) {
  u = opaque(v)  ; fresh variable u
  return(u)
}
  \end{lstlisting}

  \item Observe and rename atomically per variable, then joining atomically over multiple variables, forcing uses of the renamed variables to occur after all propendent instructions have been executed
  \begin{lstlisting}
macro enforce_map_preeval(v1, ..., vk) {
  u1 = atomic {
    w1 = opaque(v1)
    yield(w1)
  }
  ...
  uk = atomic {
    wk = opaque(vk)
    yield(wk)
  }

  x1, ..., xk = barrier(w1, ..., wk)

  return(x1, ..., xk)
}
  \end{lstlisting}

  \item Observe and rename atomically per variable, then joining atomically over multiple variables, forcing uses of the renamed variables to occur after all propendent instructions have been executed,
  ordered through a side-effect
  \begin{lstlisting}
macro enforce_map_preeval_state(v1, ..., vk) {
  u1 = atomic {
    w1 = opaque(v1)
    yield(w1)
  }
  ...
  uk = atomic {
    wk = opaque(vk)
    yield(wk)
  }

  x1, ..., xk = side_effecting_barrier(w1, ..., wk)

  return(x1, ..., xk)
}
  \end{lstlisting}

  \item Observe and rename atomically per variable, then joining atomically over multiple variables, ordered through a side-effect
  \begin{lstlisting}
macro enforce_map_nopreeval_state(v1, ..., vk) {
  u1 = atomic {
    w1 = opaque(v1)
    yield(w1)
  }
  ...
  uk = atomic {
    wk = opaque(vk)
    yield(wk)
  }
  \end{lstlisting}

  \item Side-effecting barrier
  \begin{lstlisting}
  *_ = side_effecting_barrier(w1, ..., wk) {
  return(w1, ..., wk)
  }
  \end{lstlisting}
\end{itemize}
